# Supplementary material for: Inverse solving the Schr\"odinger equation for precision alignment of a microcavity
Source: arXiv:2404.07760 source file (2024-04-11)
Supplement: Supplementary file 1 [file additional_info.tex]

In order to get single transverse modes we scan the position of the pump spot with the SLM along the ramp of the PRS until we excite a single transverse mode.
Assume we found a pump spot position that excites a single transverse mode in the PRS.
If we now continuously move that spot in one direction along the length of the PRS we will start to excite other modes as well.
If we continue moving in that direction we will eventually excite a single transverse mode again.
We reconstruct the potential for all mode patterns and calculate the corresponding tilt values by multiplying the slope of the reconstructed potentials by the cavity length, and then take a weighted average of those tilt values to get one final tilt value.
The closer a mode pattern is to a single mode the higher the weight.
Our measure of how close the system is to a single mode is the intensity minimum of adjacent intensity maxima.
For a single transverse mode those intensity minima should be zero.
When we excite multiple modes that overlap, some intensity minima will not be at zero.
The greater the excitation of multiple modes the further those minima will be away from zero.
We can give the observed mode pattern a mode quality depending on how close each intensity minimum goes to zero.
Assume we have $n$ intensity minima and let $I_\t{max}^i$ and $I_\t{max}^{i+1}$ be two adjacent intensity maxima, $\bar I_\t{max}^i$ their mean intensity, and $I_\t{min}^i$ the intensity minimum between those two maxima.
Then the  mode quality is defined as
\begin{equation}
    q = \left( 1 - \max_i{\frac{I_\t{min}^i}{\bar I_\t{max}^i}} \right) ^2,
    \label{eq:contrast}
\end{equation}
which is a number between 0 (lowest quality) and 1 (highest quality).
We take the square on the right hand side for a stronger suppression of mode patterns that are further away from a single mode.
So in order to get a tilt value of the cavity along one PRS we scan the position of the pump spot along the ramp of that PRS, reconstruct the potential for all mode patterns, fit a line through those reconstructed potentials and multiply the slopes with the cavity length, and finally average the resulting values weighted by the corresponding mode qualities.

The finer we scan the position of the pump spot the more tilt values we will get for averaging which will increase the precision of the tilt readout.
But this will in turn make the tilt acquisition slower, as the time it takes to acquire averaged tilt value is proportional to the number of different pump spot positions.
The extreme case of infinitely many positions will yield the best result, but will also take infinitely long.
The other extreme of only one pump spot position is as fast as it gets but will on average give the worst result.
One has to find a balance between having enough pump spot positions to always get at least one mode pattern that is close to a single mode, and still having a decent tilt acquisition rate.
This depends on the specific experiment at hand and the requirements of precision and speed.

We saw in the experiments that a mode quality below $\approx 75\%$ already leads to unreliable results.
Those low quality mode patterns do not increase the precision of our tilt readout and we can choose a hard threshold $q_\t{min}$ for the zero-crossings and ignore all mode patterns whose mode quality lie below this value.
In the following we will refer to mode patterns with a mode quality $q \geq q_\t{min}$ as \textit{good modes}.

A very crucial assumption of our method is that the system actually is in an energy eigenstate.
But it also happens that you do not excite only one single transverse mode, but multiple modes that are overlapping which is then not a single standing wave anymore.
In the latter case the system is not in an energy eigenstate and the wavefunction can have imaginary amplitudes.
Taking the square root of the intensity distribution to get the amplitude of the wavefunction will give unreliable results with a large standard deviation when used for potential reconstruction with our method.
We introduce two different regularization techniques to tackle this issue.
The first is the contrast (or visibility) of the intensity distribution.
For a perfect standing wave the intensity minima should go to zero.
But when there are multiple modes overlapping than the 
The second measure is the error of the linear fit of the reconstructed potential.
Since we assume linear potentials any deviations from this will lead to bigger fit errors.

In our setup $D_0$ is typically on the order of ten micrometers.
A height elevation of $\Delta d = \SI{0.1}{nm}$ over a distance of $\SI{100}{\um}$ on the mirror surface corresponds to a tilt of $\SI{1}{\micro\radian}$.
